# Supplementary material for: PDM-SSD: Single-Stage Three-Dimensional Object Detector With Point Dilation
Source: arXiv:2502.07822 source file (2025-02-10)
Supplement: Supplementary file 1 [file 06_Appendix.tex]

\section{Details of The Proposed \nickname{}}

\smallskip\noindent\textbf{(1) Detailed Network Architecture.}
% \qy{We provide the detailed architecture of our \nickname{} here. The network follows the encoder-only framework 3DSSD \cite{yang20203dssd} but has a more lightweight backbone setting. Details of the architecture on KITTI are as follows:
% }
%\yf{We provide the detailed architecture of our \nickname{} here. The backbone consists of three SA layers~\cite{qi2017pointnet++} with only two radius for query. Details of the architecture deployed on KITTI Dataset are as follows:}
\qy{Here, we provide the detailed architecture of our \nickname{}. The proposed \nickname{} has a lightweight backbone, which consists of three SA (Set Abstraction) layers~\cite{qi2017pointnet++} with only two radii for the spherical neighbor query. The detailed architecture deployed on KITTI Dataset is as follows: }
\vspace{0.2cm}

\noindent syntax: $SA(npoint, [radii], [nquery], [dimension])$
\yf{
\vspace{-0.05cm}
\begin{equation*}
\begin{aligned}
&SA(4096, [0.2,0.8], [16,32], [[16,16,32],[32,32,64]])  \\
&\rightarrow MLP(96 \rightarrow 64) \\
&SA(1024, [0.8,1.6], [16,32], [[64,64,128],[64,96,128]]) \\
&\rightarrow MLP(256 \rightarrow 128) \\
&SA(512, [1.6,4.8], [16,32], [[128,128,256],[128,256,256]]) \\
&\rightarrow MLP(512 \rightarrow 256) \\
\end{aligned}
\end{equation*}
}

\noindent where $npoint$ denotes the number of sampled points, $[radii]$ denote the grouping radii, $[nquery]$ denotes the number of grouping points, $[dimension]$ denotes the feature dimensions.

\qy{The class/centroid-aware prediction layer:}
\begin{equation*}
\begin{aligned}
&MLP(256 \rightarrow 256 \rightarrow 3) \\
\end{aligned}
\end{equation*}

The architecture of the contextual instance centroid perception module is as follows:
\begin{equation*}
\begin{aligned}
&MLP(256 \rightarrow 128 \rightarrow 3) \\
\end{aligned}
\end{equation*}

The architecture of centroid-based instance aggregation is as follows:
\yf{
\begin{equation*}
\begin{aligned}
&SA(256, [4.8,6.4], [16,32], [[356,356,512],[256,512,1024]]) \\
&\rightarrow MLP(1536 \rightarrow 512) \\
\end{aligned}
\end{equation*}
}
The final detection head is composed of two branches:
\begin{equation*}
\begin{aligned}
&\textit{cls~branch}: FC(512) \rightarrow FC(256) \rightarrow FC(256) \rightarrow FC(3)  \\
&\textit{reg~branch}: FC(512) \rightarrow FC(256) \rightarrow FC(256) \rightarrow FC(30) \\
\end{aligned}
\end{equation*}

\qy{Considering the large-scale spatial ranges and increasing number of potential instances in the Waymo and ONCE datasets, the number of sampled points are improved to 16384, 4096, 2048, and 1024 in our framework, and the contextual centroid perception boundary is improved to 2.0m. The rest of the hyperparameters are kept consistent for a fair comparison.}

\section{Additional Implementation Details}

\smallskip\noindent\textbf{(1) Data augmentation.} \qy{During training, We also apply two data augmentation strategies including scene-level augmentation and object-level augmentation. The detailed settings and hyperparameters are as follows:}

\noindent{\textbf{Scene-level augmentation:}}
% \vspace{-0.1cm}
\begin{itemize}
\setlength{\parsep}{0pt} 
\setlength{\topsep}{0pt} 
\setlength{\itemsep}{0pt}
\setlength{\parsep}{0pt}
\setlength{\parskip}{0pt}
    \item Random scene flip with a 50 $\%$ probability.
    \item Random scene rotation around $z$-axis with a random value from $[-\frac{\pi}{4}, \frac{\pi}{4}]$.
    \item Random scene scaling with a random factor from $[0.95, 1.05]$.
    % \item Transform objects (car: 20, pedestrian: 15, cyclist: 15) from other scenes, note that the internal points of all sampled objects should be over 5.
\end{itemize}

\noindent{\textbf{Object-level augmentation:}}
\vspace{-0.1cm}
\begin{itemize}
\setlength{\parsep}{0pt} 
\setlength{\topsep}{0pt} 
\setlength{\itemsep}{0pt}
\setlength{\parsep}{0pt}
\setlength{\parskip}{0pt}
    \item \qy{Transform objects from other scenes. In particular, 20 cars, 15 pedestrians, and 15 cyclists are copied to the current scene. Note that, the minimum number of points for a sampled instance is 5.}
\end{itemize}

\noindent \textbf{(2) Training and inference.}  \qy{We train the proposed \nickname{} in an end-to-end fashion with a maximum of 80 epochs. Adam solver with onecycle learning strategy \cite{smith2019super} is used for optimization. In our experiment, the batch size is set to 8, and the learning rate is set to 0.01. During inference, our \nickname{} is able to take raw point clouds and generate proposals for all objects in a single forward pass. Finally, all proposals are filtered by 3D-NMS post-processing with an IoU threshold of 0.01 on KITTI and 0.1 on Waymo/ONCE.}

% \qy{The proposed \nickname{} is built upon OpenPCDet \cite{openpcdet2020} with default settings. It trained end-to-end for a maximum epoch number of 80. We use Adam optimizer with onecycle learning strategy \cite{smith2019super}. In our experiment, the batch size is set to 8, and the learning rate is set to 0.01. During inference, our \nickname{} is able to take raw point clouds and generate proposals for all objects in a single forward pass. Finally, all proposals are filtered by 3D-NMS post-processing with an IoU threshold of 0.1.}
%\yf{We train the proposed \nickname{} end-to-end for 80 epochs with the Adam optimizer with onecycle learning strategy \cite{smith2019super}. In our experiment, the batch size is set to 8, and the learning rate is set to 0.01. During inference, our \nickname{} is able to take raw point clouds and generate proposals for all objects in a single forward pass. Finally, all proposals are filtered by 3D-NMS post-processing with an IoU threshold of 0.1 on KITTI/Waymo and 0.01 on ONCE.}

\begin{table*}[t]
  \begin{center}
      \resizebox{0.93\textwidth}{!}{   
      % \begin{tabular}{cccccc|ccc|ccc|ccc|}
      \begin{tabular}{p{16mm}<{\centering} p{16mm}<{\centering} p{16mm}<{\centering} p{16mm}<{\centering} ||p{14mm}<{\centering} |p{14mm}<{\centering} |p{14mm}<{\centering} ||p{16mm}<{\centering} |p{16mm}<{\centering} |p{16mm}<{\centering}}
\Xhline{2.0\arrayrulewidth}
      \multirow{2}{*}{$1^{st}$ layer}& \multirow{2}{*}{$2^{nd}$ layer}& \multirow{2}{*}{$3^{rd}$ layer}& \multirow{2}{*}{$4^{th}$ layer} & \multirow{2}{*}{Recall Car} & \multirow{2}{*}{Recall Ped.} & \multirow{2}{*}{Recall Cyc.} & \small{Car Mod} & \small{Ped. Mod} & \small{Cyc. Mod}  \\
      & & & & & & & (IoU=0.7) & (IoU=0.5) & (IoU=0.5)  \\
\Xhline{2.0\arrayrulewidth}
      Random & Random & Random & Random & 67.4$\%$ & 72.1$\%$ & 57.3$\%$ & 75.02  & 51.16 & 66.07 \\
      D-FPS & D-FPS & D-FPS & D-FPS & 91.4$\%$ & 69.1$\%$ & 71.6$\%$ & 78.12 & 50.46 & 65.19  \\
      D-FPS &  Feat-FPS &  Feat-FPS & Feat-FPS & 95.3$\%$ & 80.1$\%$ & 91.7$\%$ & 79.00 & 54.31 & 71.08 \\
    %   D-FPS & Ctr-aware & Ctr-aware & Ctr-aware & 75.5$\%$ & 79.2$\%$ & 78.9$\%$ & 68.05 & 54.42 & 68.67  \\
      D-FPS & D-FPS & Cls-aware & Cls-aware & 97.9$\%$ & 97.4$\%$  & 92.7$\%$ & 79.19 & 58.81 & 70.15  \\
      
      D-FPS & D-FPS & Cls-aware & Ctr-aware & 97.9$\%$ & 97.7$\%$ & 96.3$\%$ & 79.54 & 58.49 & \underline{71.33} \\
      \textbf{D-FPS} & \textbf{D-FPS} & \textbf{Ctr-aware} & \textbf{Ctr-aware} & \textbf{97.9$\%$} & \underline{\textbf{98.4$\%$}} & \textbf{97.2$\%$} & \underline{\textbf{79.57}} & \underline{\textbf{58.91}} & \textbf{71.24} \\
\Xhline{2.0\arrayrulewidth}
  \end{tabular}}
  \end{center}
  \vspace{-0.4cm}
  \caption{\revise{The correlation between the instance recall ratio and the final detection performance.}}
  \label{tab:ins_recall_detail}
  \vspace{-0.2cm}
  \end{table*}

\section{Additional Experimental Results}

\begin{table}[h]
   \centering
   \begin{minipage}[t]{0.49\textwidth}
   \begin{center}
   \resizebox{0.9\textwidth}{!}{ 
  \begin{tabular}{p{2.2cm}<{\centering}| p{1.3cm}<{\centering}| p{1.3cm}<{\centering} |p{1.3cm}<{\centering} |p{1.4cm}<{\centering} }
    \Xhline{2.0\arrayrulewidth}
   Method & 256p  & 1024p  & 4096p & 16384p \\
    \Xhline{2.0\arrayrulewidth}
    D-FPS \cite{qi2019deep} & \textless 0.1 ms & 0.5 ms & 2.8 ms & 23.7 ms \\
    Feat-FPS \cite{yang20203dssd} & 0.3 ms & 0.7 ms & 4.2 ms & 40.6 ms \\
    \textbf{Cls/Ctr-aware} & \textbf{0.2 ms} & \textbf{0.2 ms} & \textbf{0.3 ms} & \textbf{0.5 ms}  \\
%   Memory Consumption (MB) & 478 & 980 & 544  \\
%   Speed (\todo{fps}) & 56  & 40 & 48  \\
    \Xhline{2.0\arrayrulewidth}
   \end{tabular}}
   \end{center}
   \vspace{0.1cm}
%   \caption{The computational memory consumption of different sampling methods.}
   \end{minipage}
   
\vspace{-0.2cm}
   \begin{minipage}[t]{0.49\textwidth}
   \begin{center}
   \resizebox{0.9\textwidth}{!}{ 
%   \begin{tabular}{c|c|c|c|c|c}
  \begin{tabular}{p{2.2cm}<{\centering}| p{1.3cm}<{\centering}| p{1.3cm}<{\centering} |p{1.3cm}<{\centering} |p{1.4cm}<{\centering} }
    \Xhline{2.0\arrayrulewidth}
   Method & 256p & 1024p & 4096p & 16384p \\
    \Xhline{2.0\arrayrulewidth}
    D-FPS \cite{qi2019deep} & \textless 1 MB & \textless 1 MB & \textless 1 MB & \textless 1 MB \\
    Feat-FPS \cite{yang20203dssd} & 64 MB & 104 MB & 448 MB & 6228 MB \\
    \textbf{Cls/Ctr-aware} & \textbf{0.25 MB} & \textbf{1 MB} & \textbf{4 MB} & \textbf{17 MB}  \\
%   Memory Consumption (MB) & 478 & 980 & 544  \\
%   Speed (\todo{fps}) & 56  & 40 & 48  \\
    \Xhline{2.0\arrayrulewidth}
   \end{tabular}}
   \end{center}
   \end{minipage}
%   \vspace{-0.2cm}
   \caption{\revise{Time and memory consumption of sampling methods.}}
   \label{tab:effi_sample}
  \vspace{-0.3cm}
   \end{table}

\smallskip\noindent\textbf{(1) Preserving more foreground points really benefits the final detection performance?}  As mentioned in section \ref{subsec:instance-aware downsampling strategy}, two instance-aware strategies are proposed to keep high instance recall while hierarchically downsampling the points. However, it remains unclear that whether the more foreground points really benefit the final detection performance. To this end, we further justify the motivation of our \nickname{} here. Specifically, we conduct several groups of experiments based on our framework with different sampling strategies. Note that, the network architecture and parameter settings are kept consistent. The quantitative detection results, accompanied with the instance recall ratio after the last downsampling layers by using different possible combinations of the sampling approaches are shown in Table \ref{tab:ins_recall_detail}.

\qy{From the results in Table \ref{tab:ins_recall_detail} we can see that: (1) the instance recall ratio is positively correlated with the final detection performance, especially for small objects with a limited number of points such as \textit{pedestrians} and \textit{cyclists}. (2) The detection performance of \textit{cars} is relatively robust to the variations of sampling strategies, primarily because that \textit{car} usually has a sufficient number of foreground points remaining after downsampling, hence relatively easy to be detected. (3) Adopting the proposed instance-aware sampling strategies at the early encoding layers may negatively affect the final detection performance, primarily because of the insufficient semantic information in the early latent point features. (4) Deploying the proposed instance-aware downsampling strategies at the last two encoding layers can significantly improve the detection performance. Overall, this experiment further demonstrates that more foreground points are appealing for object detection task, especially for small but important objects.
}

\smallskip\noindent\textbf{(2) Efficiency of Sampling.}  
We further explore the efficiency of different sampling strategies, to have an intuitive idea of the advantages of our instance-aware sampling. Table~\ref{tab:effi_sample} compares the time and memory consumption of different sampling strategies with a varying number of points. 
% Note that, we only change the sampling strategies while keeping all other modules unchanged. 
We can clearly see that the proposed instance-aware sampling has superior efficiency compared with the Feat-FPS \cite{yang20203dssd}, hence leading to a higher frame rate of our method during inference.
%\qy{From the results in Table \ref{tab:ins_recall_detail} we can also see that: {1) Adopting the proposed instance-aware sampling strategies at the early encoding layers may negatively affect the final detection performance, primarily because of the insufficient semantic information in the early latent point features.} 2) Deploying the proposed instance-aware downsampling strategies at the last two encoding layers can significantly improve the detection performance. Additionally, adopting the centroid-aware sampling at the final encoding layer is likely to achieve slightly better results, since the last feature map is quite sparse and informative. Preserving more centroid points is likely to ease the difficulty in the centroid perception module. }

%\qy{From the results in Table \ref{tab7} we can see that: /todo{1) Adopting the proposed instance-aware sampling strategies at the early encoding layers may negatively affect the final detection performance, primarily because of the insufficient semantic information in the early latent point features.} 2) Deploying the proposed instance-aware downsampling strategies at the last two encoding layers can significantly improve the detection performance. Additionally, adopting the centroid-aware sampling at the final encoding layer is likely to achieve slightly better results, since the last feature map is quite sparse and informative. Preserving more centroid points is likely to ease the difficulty in the centroid perception module. }

\smallskip\noindent\textbf{(3) Evaluation on KITTI validation set.} \qy{We also report the detection results achieved by several representative approaches on the \textit{validation} set of the KITTI Dataset in Table \ref{tab:kitti_val_pcdet}. Note that, all results achieved by baselines are reproduced based on the OpenPCDet\footnote{https://github.com/open-mmlab/OpenPCDet}. In particular, all baselines are trained with multi-class objects in a single model for a fair comparison. It can be seen that our single-stage \nickname{} achieves superior detection performance compared with other point-based baselines. We also noticed that the prior SoTA detector 3DSSD\footnote{https://github.com/qiqihaer/3DSSD-pytorch-openPCDet} achieve poor results on the class of pedestrian and cyclist, further demonstrating the advantages of our \nickname{}.}

\smallskip\noindent\textbf{(4) Efficiency of our \nickname{} on large-scale LiDAR scenarios.} To further verify the efficiency of our \nickname{} on large-scale 3D datasets, we further report the efficiency of our \nickname{} on the validation set of Waymo and ONCE datasets. As shown in Table~\ref{tab:effi_waymo&once}, the proposed \nickname{} can still achieve satisfactory real-time performance in such complex panoramic scenes.

%\smallskip\noindent\textbf{(3)Efficiency performance on challenging large-scale LiDAR scenarios.} To further certify the efficiency and adaptation on advance LiDAR sensors, we also illustrate efficiency details on Waymo and ONCE \textit{validation} set. As shown in Table~\ref{tab:effi_waymo&once}, our \nickname{} still have capacity of keeping light-weight and efficient even in complicated panoramic scenes.

\begin{table}[t]
   \begin{center}
      \resizebox{0.48\textwidth}{!}{   
      \begin{tabular}{c|r|c||p{14mm}<{\centering}|p{14mm}<{\centering}|p{14mm}<{\centering}}
    %   \begin{tabular}{p{4mm}<{\centering} |p{26mm}<{\centering} |p{20mm}<{\centering} |p{18mm}<{\centering} |p{18mm}<{\centering} |p{18mm}<{\centering}}
\Xhline{2.0\arrayrulewidth}
      \multirow{2}{*}{} & \multirow{2}{*}{Method} & \multirow{2}{*}{Type} & \small{Car Mod} & \small{Ped. Mod} & \small{Cyc. Mod}  \\
      % & & & & & & & Easy & Mod. & Hard & Easy & Mod. & Hard & Easy & Mod. & Hard  \\
      & & &  (IoU=0.7) & (IoU=0.5) & (IoU=0.5)  \\
\Xhline{2.0\arrayrulewidth}
    %   \multirow{3}{*}{\rotatebox{90}{Voxel-based}}
      \multirow{3}{*}{Voxel-based}
      & SECOND \cite{yan2018second}   & 1-stage  & 78.62 & 52.98 & 67.15  \\
      & PointPillars \cite{lang2019pointpillars}   & 1-stage  & 77.28  & 52.29 & 62.28  \\
      & Part-$A^2$  \cite{shi2020points}    & 2-stage  & 79.40  & \underline{60.05} & 69.90  \\
\Xhline{1.0\arrayrulewidth}
      \multirow{1}{*}{Point-Voxel}
      & PV-RCNN  \cite{shi2020pv} & 2-stage & \underline{83.61}  & 57.90 & 70.47  \\
\Xhline{1.0\arrayrulewidth}  
      \multirow{3}{*}{Point-based}
      & PointRCNN \cite{shi2019pointrcnn} & 2-stage & 78.70 & 54.41 & \underline{72.11}  \\
      & 3DSSD \cite{yang20203dssd}    & 1-stage  & 79.06 & 10.49 & 16.93  \\ % 
% \Xhline{2.0\arrayrulewidth}
\cline{2-6}
% \Xhline{1.0\arrayrulewidth}
      & \textbf{\nickname{} (Ours)} & \textbf{1-stage} & \textbf{79.57} & \textbf{58.91} & \textbf{71.24}  \\
\Xhline{2.0\arrayrulewidth}
   \end{tabular}}
   \end{center}
   \vspace{-0.2cm}
   \caption{Performance comparison of different detectors based on the OpenPCDet library. Note that, all detectors are trained with multi-class objects together, and the results are achieved by using a single detection model.}
   \label{tab:kitti_val_pcdet}
%   \vspace{-0.3cm}
   \end{table} 
   
\begin{table}[t]
    \centering
    \scalebox{0.8}{
    \begin{tabular}{r|r|r|r|r|r}
    \Xhline{2.0\arrayrulewidth}
        Dataset   & \tabincell{c}{\textit{Mem.}}   & \tabincell{c}{\textit{Paral.}} &\tabincell{c}{\textit{Speed$^{\bot}$}}  & \tabincell{c}{\textit{Speed$^{\top}$}} & \tabincell{c}{\textit{Input Scale}}   \\
    \Xhline{2.0\arrayrulewidth}
        Waymo~\cite{sun2020scalability}       & 626 MB    & 16    & 9$^{\dagger}$     & 14           & 81920    \\
                    & 433 MB    & 23    & 8$^{\dagger}$     & 20           & 65536    \\
    \Xhline{1.0\arrayrulewidth}
        ONCE~\cite{mao2021one}        & 401 MB    & 25    & 11$^{\dagger}$    & 21           & 60k    \\
    \Xhline{2.0\arrayrulewidth}
    \end{tabular}
    }
    % \vspace{-0.2cm}
    \caption{\qy{Efficiency of our \nickname{} on Waymo and ONCE Datasets. The number of input points to our framework is increased,  considering the large-scale panoramic scenes compared with KITTI. Here ``Mem.'' and ``Paral.'' denote the GPU memory footprint per frame during inference and the maximum number of batches that can be parallelized on one RTX2080Ti~(11GB). ''Speed$^{\bot}$'', ''Speed$^{\top}$'' is inference speed when processing one frame or full-loaded GPU memory. $^{\dagger}$ We divide the whole scene into four parallel parts in the first sampling layer.}}
    \label{tab:effi_waymo&once}
    \vspace{-0.3cm}
\end{table}

\smallskip\noindent\textbf{(5) Qualitative visualization of our instance-aware downsampling. }\qy{To intuitively compare the performance of different sampling approaches, we qualitatively show the visualization of the downsampled point clouds achieved by different approaches in Figure \ref{fig:visual_downdsample}. Clearly, the proposed instance-aware sampling can effectively preserve more foreground points (shown in red), especially for foreground points belonging to small and sparse instances (\textit{e.g.,} \textit{pedestrian}), as well instances far away from the sensors.}

\smallskip\noindent\textbf{(6) Visualization of the Contextual Centroid Perception.} \qy{We also visualize the results produced by our contextual centroid perception module in Figure \ref{fig:visual_context_centroid}. It is clear that the downsampled point clouds at this stage are quite sparse and insufficient, which makes the centroid estimation and instance regression considerably difficult. Therefore, it is necessary to exploit the useful information around the instance, even outside the ground-truth bounding boxes. Thanks to the proposed contextual centroid perception module, our \nickname{} can even precept the objects with extremely indistinguishable geometry and limited points (shown in purple dotted circles). This further demonstrated the effectiveness of the proposed module.}

\smallskip\noindent\textbf{(7) Additional qualitative detection results on the KITTI Dataset.} \qy{We also show extra qualitative detection results achieved by our \nickname{} on the \textit{validation} (Figure \ref{fig:visual_kitti_val}) and \textit{test} (Figure \ref{fig:visual_kitti_test}) split of the KITTI Dataset. It can be seen that our \nickname{} can achieve satisfactory detection performance on this dataset, even for some challenging cases. It is also worth mentioning that the detection results of different objects are achieved by our \nickname{} in a single pass, instead of the common practice to train separate models for different objects.}

\smallskip\noindent\textbf{(8) Additional qualitative detection results on the large-scale datasets.} Here, we present extra qualitative detection results achieved by our \nickname{} on two large-scale datasets with challenging panoramic scenarios. Figure~\ref{fig:visual_waymo_val} and Figure~\ref{fig:visual_once_val} illustrate the detection results on the validation set of Waymo and ONCE Dataset respectively. It can be seen that our \nickname{} can also achieve promising detection performance in challenging and complex 3D scenes. 

% \section{Limitation and Future Work}
% \smallskip\noindent\textbf{Limitation.} Although the proposed \nickname{} can achieve remarkable efficiency in object detection of large-scale LiDAR points clouds, it also has limitations. \textit{e.g.,} the instance-aware sampling relies on the semantic prediction of each point, which is susceptible to class imbalances distribution. For future work, we will further explore advanced techniques to alleviate the imbalanced issue.

\section{Potential Negative Societal Impact}
\qy{In this paper, we proposed an efficient point-based solution capable of achieving promising low-cost objects detection in autonomous driving scenarios. Our model is trained and evaluated totally based on open-sourced datasets, and there is no known potential negative impact on society.}

\section{Video Illustration}
We provide a video demo illustrating the detection performance of our IA-SSD in 3D point clouds, which can be viewed at \url{https://youtu.be/3jP2o9KXunA}.

\clearpage

\begin{figure*}[thb]
   \centering
   \includegraphics[width=1.0\textwidth]{figs/fig4_visual_downdsample.pdf}
    \caption{\qy{Qualitative visualization of the downsampled point clouds achieved by different sampling strategies (From left to right, D-FPS, F-FPS, and the proposed instance-aware sampling). Note that, the raw point clouds and representative points are colored in white and gold, respectively. Positive representative points are highlighted in red.}}
   \label{fig:visual_downdsample}
   \vspace{-0.5cm}
\end{figure*}

\begin{figure*}[h]
   \centering
   \includegraphics[width=1.0\textwidth]{figs/fig5_visual_context_centroid.pdf}
    \vspace{-0.2cm}
    \caption{\qy{Visualization of the contextual centroid perception on the \textit{validation} spit of the KITTI dataset. All representative points and predicted centroid are colored in gold and red, respectively. In particular, we also show the offsets of representative points inside/around the objects in red/gold. Best viewed in color.}}
   \label{fig:visual_context_centroid}
   \vspace{-0.3cm}
\end{figure*}

\begin{figure*}[h]
   \centering
    \includegraphics[width=1.0\textwidth]{figs/fig6_visual_kitti_val_1.pdf}
    \caption{\qy{Extra qualitative results achieved by our \nickname{} on the \textit{validation} set of the KITTI Dataset. We also show the corresponding projected 3D bounding boxes on images. Note that, the ground-truth bounding boxes are shown in red, and the predicted bounding boxes are shown in green for \textit{car}, cyan for \textit{pedestrian}, and yellow for \textit{cyclist}. Best viewed in color.}}
   \label{fig:visual_kitti_val}
\end{figure*}

\begin{figure*}[h]
   \centering
   \includegraphics[width=1.0\textwidth]{figs/fig7_visual_kitti_test.pdf}
    \caption{\qy{Extra qualitative results achieved by our \nickname{} on the \textit{test} set of the KITTI Dataset. We also show the corresponding projected 3D bounding boxes on images. Note that, there is no ground-truth bounding boxes available, hence we only show the predicted bounding boxes in green for \textit{car}, cyan for \textit{pedestrian}, and yellow for \textit{cyclist}. The centroid predictions are marked in red, while the 256 representative points are shown in gold. Best viewed in color.}}
   \label{fig:visual_kitti_test}
\end{figure*}

\begin{figure*}[thb]
   \centering
   \includegraphics[width=0.92\textwidth]{figs/fig8_visual_waymo.pdf}
    \caption{\yf{Extra qualitative results achieved by our \nickname{} on the \textit{val} set of the Waymo Dataset. Here We demonstrate our detection results on some challenging scenes. Note that, the ground-truth bounding boxes are shown in red, and the predicted bounding boxes are shown in green for \textit{vehicle}, cyan for \textit{pedestrian}, and yellow for \textit{cyclist}. Best viewed in color.}}
   \label{fig:visual_waymo_val}
\end{figure*}

\begin{figure*}[thb]
   \centering
   \includegraphics[width=0.92\textwidth]{figs/fig9_visual_once.pdf}
    \caption{\yf{Extra qualitative results achieved by our \nickname{} on the \textit{val} set of the ONCE Dataset. Here We demonstrate our detection results on some challenging scenes. Note that, the ground-truth bounding boxes are shown in red, and the predicted bounding boxes are shown in green for \textit{vehicle}, cyan for \textit{pedestrian}, and yellow for \textit{cyclist}. Best viewed in color.}}
   \label{fig:visual_once_val}
\end{figure*}
